# Supplementary material for: Roundtable Policy: Confidence-Weighted-Consensus Aggregation Improves Multi-Agent-System Reasoning
Source: arXiv:2509.16839 source file (2026-11-23)
Supplement: Supplementary file 1 [file supp_labels.tex]

\makeatletter
\xr@def{S}{app:bench}{2}
\xr@def{S}{app:kendall}{1.3}
\xr@def{S}{app:mas}{4}
\xr@def{S}{app:notation}{1}
\xr@def{S}{app:significance}{1.2}
\xr@def{S}{appendix_dataset}{2.4}
\xr@def{S}{fig:fusio_singletask}{13}
\xr@def{S}{fig:grader_consistency}{7}
\xr@def{S}{fig:grader_multitask}{10}
\xr@def{S}{fig:grader_singletask}{11}
\xr@def{S}{fig:improvement_multitask}{2}
\xr@def{S}{fig:improvement_singletask}{4}
\xr@def{S}{fig:mse_dataset}{1}
\xr@def{S}{fig:multitask_gain_all}{3}
\xr@def{S}{fig:player_multitask}{12}
\xr@def{S}{fig:player_singletask}{9}
\xr@def{S}{fig:rank_dist}{6}
\xr@def{S}{fig:singletask_gain_all}{5}
\xr@def{S}{sup:graders}{3.3}
\xr@def{S}{sup:multi-performance}{3.1}
\xr@def{S}{sup:single-performance}{3.2}
\xr@def{S}{tab:TaskBench}{2}
\xr@def{S}{tab:course_names}{6}
\xr@def{S}{tab:dataset_comparison}{3}
\xr@def{S}{tab:model_notation}{1}
\xr@def{S}{tab:multitask_wilcoxon_1_5}{7}
\xr@def{S}{tab:multitask_wilcoxon_6_9}{8}
\xr@def{S}{tab:profiling}{4}
\xr@def{S}{tab:singletask_wilcoxon_1_5}{9}
\xr@def{S}{tab:singletask_wilcoxon_6_9}{10}
\xr@def{S}{tab:subdomain_mapping}{5}
\makeatother
